# Supplementary material for: Pixel-Aligned Non-parametric Hand Mesh Reconstruction
Source: arXiv:2210.09198 source file (2022-10-17)
Supplement: Supplementary file 1 [file appendix.tex]

\section{Additional Network Details}
\subsection{Spiral Operator}
\par In our mesh decoder, we use the spiral operator~\citep{spiralnet++} to process vertex features in the spatial domain. The spiral operator defines a spiral selection of neighbors for a center vertex $\vertex$ by imposing the order on elements of the $k-$disk. A $k-$ring and a $k-$disk around a center vertex $\vertex$ can be defined as follows:
\begin{equation}
\begin{split}
    0-ring(\vertex)&={\vertex}, \\
    k-disk(\vertex)&=\bigcup_{i=0...k}i-ring(\vertex), \\
    (k+1)-ring(\vertex)&=\neighborset(k-ring(\vertex))  \textbackslash  k-disk(\vertex).\\
\end{split}
\end{equation}
where $\neighborset(\vertices)$ denotes the vertex neighborhood. 
\par The spiral length is denoted as $\seq$, then we can get an ordered set $\seqorder(\vertex, \seq)$ consisting of $\seq$ vertices by concatenating of $k-$rings:
\begin{equation}
\begin{split}
    \seqorder(\vertex, \seq) \subset (0-ring(v), 1-ring(v),...,k-ring(v)). \\
\end{split}
\end{equation}
\par After getting the sequence, we can define the convolution in the manner of the euclidean convolution. The spiral convolution operator for a node $i$ can be defined as:
\begin{equation}
\begin{split}
    \meshfeature_{\stage + 1} ^ i = \gamma_{\stage + 1}(\parallel_{j \in S(i, \seq)}\meshfeature_{\stage} ^ j)
\end{split}
\end{equation}
where $\gamma$ is MLPs and $\parallel$ denotes the concatenation operation.

\subsection{Mesh Sampling}
\par We apply a multi-scale hand mesh representation to capture both global and local information. At each stage of the mesh decoder, the number of mesh vertices are changed by the factor of 2. We follow COMA~\citep{ranjan2018generating} to perform the in-network sampling operations(down-sampling and up-sampling) using pre-computed transform matrices. The down-sampling matrix $\downsampling$ is obtained by iteratively contracting mesh vertex pairs while maintaining surface error approximation using quadric metrics. The up-sampling matrix $\upsampling$ is obtained by including barycentric coordinates of the vertices which are discarded during the downsampling. 
% For the vertex node feature $\meshfeature \in  \mathbb{R}^{N*C}$
\begin{table}[!htbp]
  \caption{\small Analysis on different backbones, evaluated on FreiHAND. All backbones are pre-trained on ImageNet.}
  \label{compare backbone}
  \begin{center}
  \begin{tabular}{lll}
    \multicolumn{1}{c}{Backbone} &\multicolumn{1}{c}{PA-MPJPE$\downarrow$} &\multicolumn{1}{c}{PA-MPVPE$\downarrow$}
        \\ \hline \\
    HRNet-W64 &6.4 &6.5\\
    ResNet-50   &6.7 &6.9\\
  \end{tabular}
\end{center}
\end{table}
\subsection{Network Architecture details}
% The 2D feature extractor constitutes of ResNet50 followed by a series of deconvolution layers to obtain multi-scale feature maps
\par For the feature encoder, we adopt different backbones including HRNet-W64~\citep{hrnet} and ResNet-50~\citep{resnet}. The backbone is followed by a series of deconvolution layers to obtain multi-scale feature maps $\downsampledfeature_\stage$ and $\upsampledfeature_ \stage$. The feature maps of the same stage have the same channels and sizes \emph{i.e.} 2048$\times$7$\times$7, 1024$\times$14$\times$14, 512$\times$28$\times$28, 256$\times$56$\times$56. We employ four 1$\times$1 convolution layers to get $\imagefeature \in \{512\times7\times7, 256\times14\times14, 128\times28\times28, 64\times56\times56\}$. The feature maps are then passed to four mesh decoding blocks. The output channels of each block are the same as $\imagefeature$ size in each stage $\stage$. A block consists of a spiral convolution layer and a self-attention module. For the spiral convolution, we set the spiral length $\seq$ as 27. For the self-attention module, we set the number of heads to 4.
\par We study the behavior of different encoder backbones. Both HRNet~\citep{hrnet} and ResNet~\citep{resnet} model are pre-trained on the ImageNet. In table~\ref{compare backbone}, we find that HRNet has greater performance than using ResNet-50. As HRNet uses high-resolution feature pyramids, we observe further improvement.
% For each backbone, we extract feature maps of the same size.
\begin{figure}[!t]
  \centering
  \includegraphics[width=\textwidth,trim={0 0.2cm 0 0cm},clip]{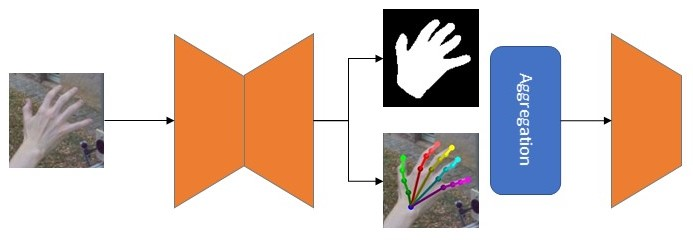}
  \caption{\small The re-designed 2D image feature extractor.}
  \label{new_2d_extractor}
\end{figure}
\subsection{The re-designed 2D feature extractor for GCN}
\par Inspired by \citep{handmesh}, we propose to add semantic aggregation to our 2D feature extractor. Specifically, we combine all the predicted joint heatmaps to aggregate 2D joint locations, which can take advantage of our 2D auxiliary tasks. Then, we use another backbone to encode the combined heatmaps and exploit the feature maps as previous settings. \Figref{new_2d_extractor} shows the pipeline.
\begin{figure}[!htbp]
  \centering
  \includegraphics[width=0.75\textwidth,trim={0 0cm 0 0cm},clip]{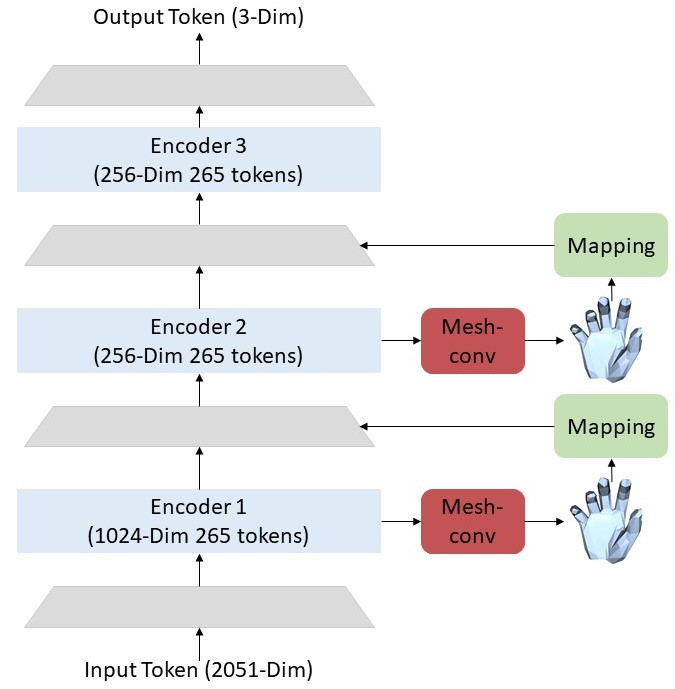}
  \caption{\small Architecture of transformer-based method.}
  \label{fig_transformer_based}
\end{figure}
\section{Architecture of Transformer-based method}
\par We inject our feature mapping and the hierarchical decoding into the Multi-Layer transformer encoder~\citep{metro}. Given the joint and mesh vertex queries, the encoder maps the input to 3D hand joints and mesh vertices.
\par As shown in \Figref{fig_transformer_based}, the encoder consists of three blocks. All three blocks have the same number of tokens. The hidden dimensions are 1024, 256, and 64. For the first two blocks, we use two additional mesh-conv layers to predict intermediate mesh results. The pixel-aligned features with the same dimension as blocks are obtained using the mapping module and then concatenate to mesh features.
\section{Failure Cases}
\par \Figref{fig_failure} shows three typical failure cases of our method. In the first row, when the hand is severely occluded and the hands are not bounded by the crop size,  some parts of the hand out of the image, our method fails to recover a correct hand mesh. In the second row, we observe when only a small portion of the hand is visible, our method predicts the wrong 2D pose and silhouette as well as the hand mesh. Referring to the last row, although the overall shape seems to be reasonable, it is difficult to obtain an accurate 3D mesh due to the heavy self-occlusion. The self-occlusion is one of the biggest challenges for 3D hand mesh reconstruction or pose estimation.
\begin{figure}[!htbp]
  \centering
  \includegraphics[width=\textwidth,trim={0 1cm 0 0cm},clip]{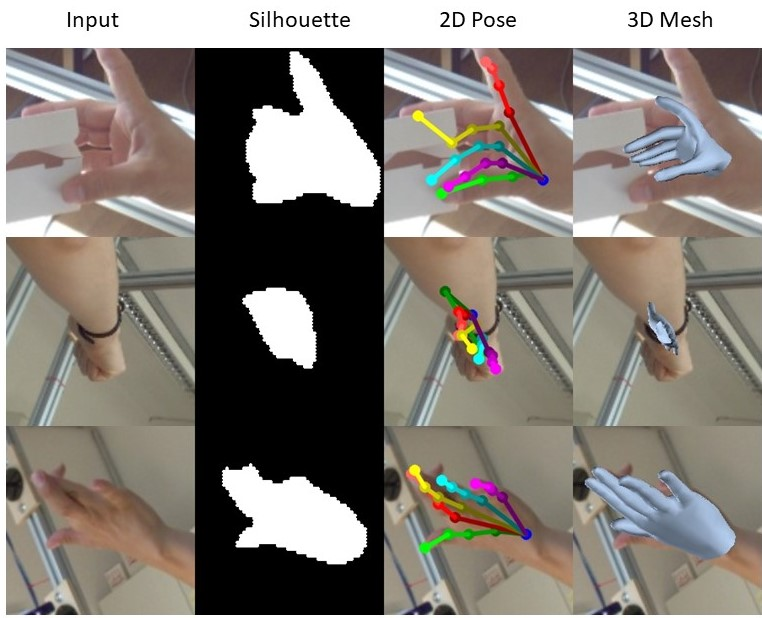}
  \caption{\small Failure cases of our method.}
  \label{fig_failure}
\end{figure}

\section{Additional Results}
\subsection{Full result comparison on FreiHAND testset}
\par As a supplement to our result on the FreiHAND testset, \Figref{fig_pck} plots PCK curves of 3D joints and 3D mesh vertices. The curve of our method achieves state-of-the-art for hand mesh reconstruction on the FreiHAND dataset.
\begin{figure}[!htbp]
  \centering
  \includegraphics[width=\textwidth]{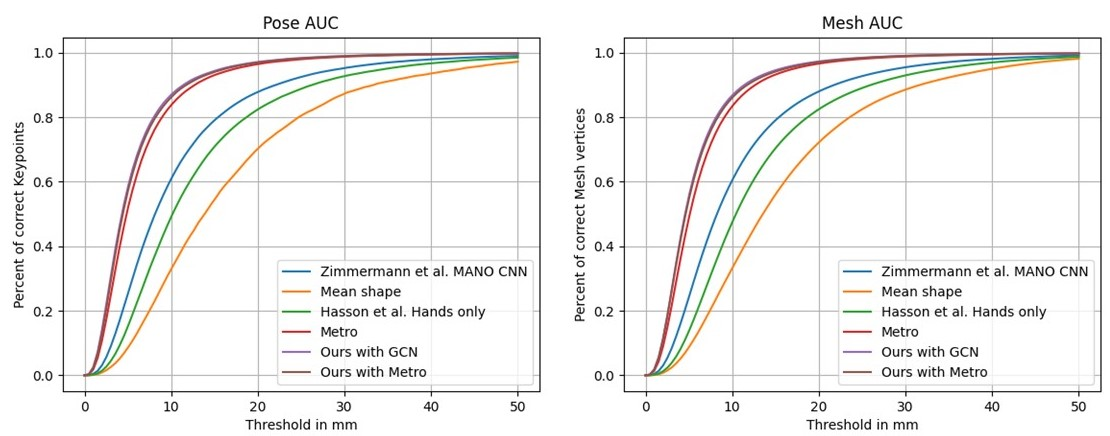}
  \caption{\small The pose and mesh AUC curve comparison with the state-of-the-art methods on the FreiHAND dataset.}
  \label{fig_pck}
\end{figure}
\subsection{Additional Qualitative Results}
\par \Figref{fig_examples} illustrates the comprehensive qualitative results of our method. The challenges of the input include complicated hand poses and hand-object interaction situations. Overcoming these difficulties, our method can predict accurate hand mesh as well as silhouette and 2D pose.
\begin{figure}[!htbp]
  \centering
  \includegraphics[width=\textwidth,trim={1.2cm 0.1cm 0 0}, clip]{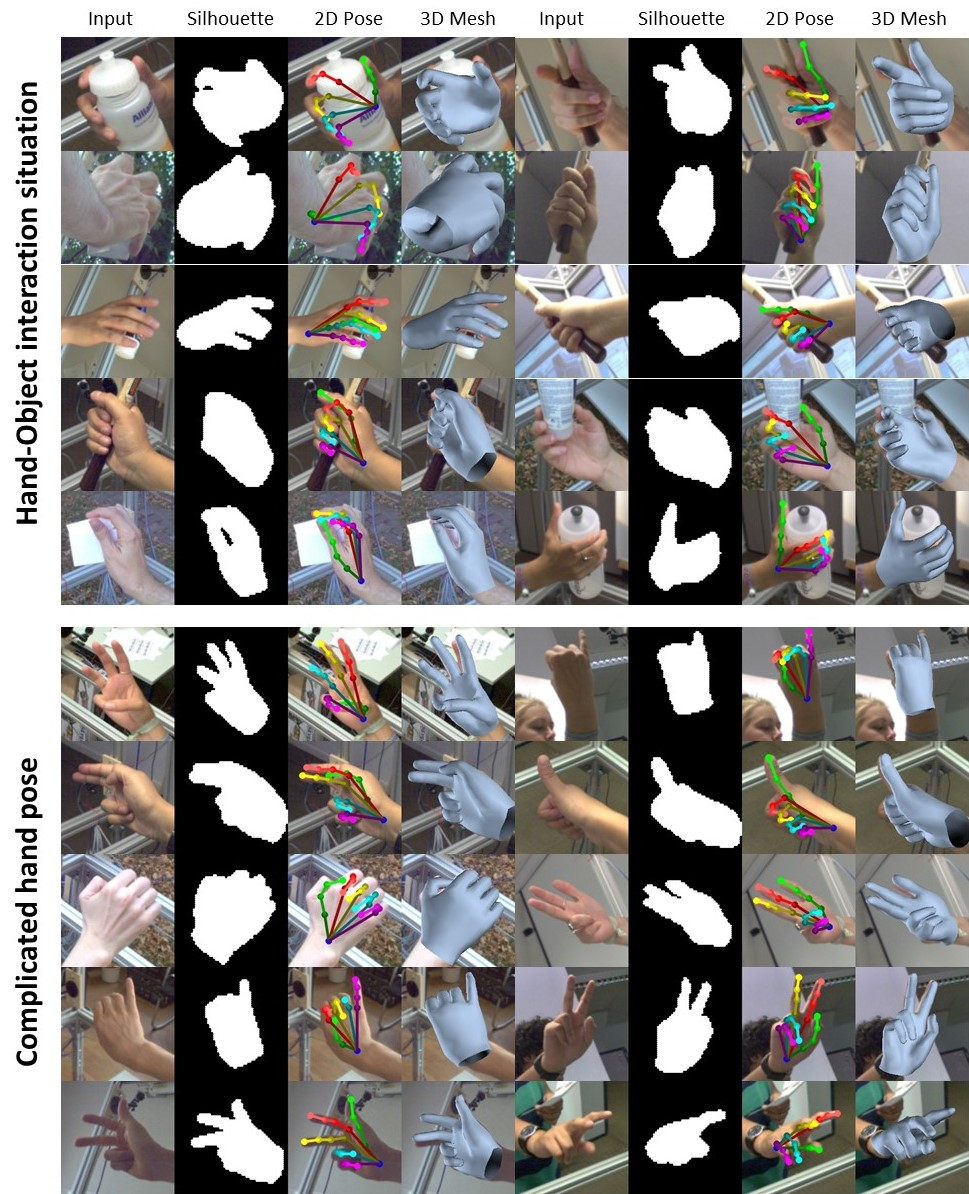}
  \caption{\small Qualitative results on FreiHAND dataset.}
  \label{fig_examples}
\end{figure}
